# Supplementary material for: Implicit Hypergraph Neural Network
Source: arXiv:2508.14101 source file (2025-12-01)
Supplement: Supplementary file 1 [file appendix.tex]

%\begin{comment}

% Second table

\begin{comment}
\begin{figure*}[h!]
    \centering
    \begin{subfigure}[b]{0.48\textwidth}
        \centering
        \includegraphics[width=\textwidth]{figs/tsne_502.png}
        \caption{}
        \label{fig:sub1}
    \end{subfigure}
    \hfill
    \begin{subfigure}[b]{0.48\textwidth}
        \centering
        \includegraphics[width=\textwidth]{figs/tsne_503.png}
        \caption{}
        \label{fig:sub2}
    \end{subfigure}
    \hfill
    \begin{subfigure}[b]{0.48\textwidth}
        \centering
        \includegraphics[width=\textwidth]{figs/tsne_504.png}
        \caption{}
        \label{fig:sub3}
    \end{subfigure}
    \hfill
    \begin{subfigure}[b]{0.48\textwidth}
        \centering
        \includegraphics[width=\textwidth]{figs/tsne_50ihnn11.png}
        \caption{}
        \label{fig:sub4}
    \end{subfigure}
    \caption{T-SNE embedding visualization for 3-layer HGNN (top left), 4-layer HGNN (top right), 5-layer HGNN (bottom left) and IHNN (bottom right).}
    \label{fig:embedding_my}
\end{figure*}
\end{comment}
